# Supplementary material for: Incentive-aware Contextual Pricing with Non-parametric Market Noise
Source: arXiv:1911.03508 source file (2023-02-07)
Supplement: Supplementary file 1 [file A2_AppendixFullInfo.tex]

\label{appsec:fullinforoadmap}
%We start with a f
To show that
 the $T$-period regret of Algorithm \ref{algo:fullinfo} is upper bounded as
$\reg (T)  =  \mathcal{O}\left(\sqrt{dN^3 T\log(T)}\right)$, we will makes use of the following events throughout our proof:
\begin{align}
    & \xi_t := \Big\{\norm{\widehat{\beta}_t - \beta}_1 \leq \frac{\delta_t}{x_{\max}} \Big\} ~~ \text{where}~~ \delta_{t} = \frac{4\sqrt{d\log(t-1)}\epsilon_{\max} x_{\max}^2}{\lambda_0^2\sqrt{N(t-1)}} \label{eq:full:good_event}\\ 
    & \xi_t^- :=  \left\{\left|F^-({z})-  \widehat{F}_t^-({z}) \right| \leq \gamma_t + 2c_f N^2\delta_t , ~~ \forall {z} \in \R \right\} \label{eq:full:event_F-} \\
    & \xi_t^+ :=  \left\{\left|F^+({z})-  \widehat{F}_t^+({z}) \right| \leq \gamma_t + c_f N \delta_t, ~~ \forall {z} \in \R\right\}\,,\label{eq:full:event_F+}
\end{align}
 where $\gamma_t := {\sqrt{2\log(t)}}/{\sqrt{t}}$, $\lambda_0^2$ is the minimum eigenvalue of covariance matrix $\Sigma$, and $c_f  = \sup_{z \in [-\epsilon_{\max}, \epsilon_{\max}]} f(z)$. Under event $\xi_t$, the estimation error in the mean vector is small, and under event $\xi_t^-$  and $\xi_t^+$, the estimation errors in $F^-$ and $F^+$ are small respectively. Furthermore, we note that under these events, our estimates for $\beta$, $F^-$, and $F^+$ become more accurate as we obtain more data points over time. We now define a threshold time period $\TT$, starting from which 
our estimates are ``sufficiently accurate'':
\begin{align}
    \label{eq:defTT}
    \TT = \left \lceil \max\left\{ \sqrt{dT}, \frac{16 x_{\max}^2\log(T)}{\lambda_0^2},2\right\} \right \rceil+ 1 = \mathcal{O}(\sqrt{dT})\,.
\end{align}
 We will later discuss the significance of this construction for $\TT$.

  For simplicity, we let $y_t := \langle \beta, x_t \rangle$, and $\widehat{y}_t := \langle  \widehat{\beta}_t, x_t \rangle$. %We further show that under event $\xi^t$, for any $v \in [\underline{r}_t, \max\{r_t, r_t^\star\}]$, the price margins and their estimates are well behaved, i.e., they both fall in an desirable interval $H$, which will be defined later. Note that price margin and its estimate at valuation $v$ is defined as $v- \langle \beta, x_t\rangle$ and $ v- \langle \widehat{\beta}_t, x_t\rangle$, respectively.
  Then, assuming that buyers are always truthful, the regret in period  $t$ is given by 
\begin{align}
\label{eq:full:R_t0}
    \reg_t ~ = ~ & \expect\left[\text{REV}^\star_t - \rev_t(r_t) \right] \nonumber\\
    %  ~ = ~ & \expect\left[\expect\left[\rev_t(r_t^\star) - \rev_t(r_t) ~ \Big| ~ x_t\right]\right] \nonumber\\
     ~ = ~ & \expect\left[\int_{0}^{r_t^\star} F^-({z}-y_t)d{z} - r_t^\star \left[ F^+(r_t^\star-y_t)\right] - \int_{0}^{r_t} F^-({z}-y_t)d{z} + r_t \left[ F^+(r_t-y_t)\right]\right]
    %   ~ := ~ & \expect\left[\mathcal{R}_t \right] 
      \,,
\end{align}
where the expectation is taken with respect to $x_t \sim \mathcal{D}$ and $r_t$; the second equality follows from Proposition \ref{prop:benchmark}.  Define 
 \begin{align}
     & \mathcal{R}_t := \int_{0}^{r_t^\star} F^-({z}-y_t)d{z} - r_t^\star \left[ F^+(r_t^\star-y_t)\right] - \int_{0}^{r_t} F^-({z}-y_t)d{z} + r_t \left[ F^+(r_t-y_t)\right]  ~~\text{and}~~\\
    & \rho_t({r},y,F^{(1)},F^{(2)}) := \int_{0}^{r} F^{(2)}({z}-y)d{z} - r \left[ F^{(1)}({r}-y)\right]  \label{eq:defrho}
    \,.
\end{align}

% \paragraph{Additional Notation} Here, we introduce some additional notation. Let $\expect_{\epsilon_t}[\cdot]$ be the expectation taken with respect to $\{\epsilon_{i,t}\}_{ i\in [N]}$. We define $y_t := \langle \beta, x_t \rangle $, $\widehat{y}_t := \langle \widehat{\beta}_\ell, x_t \rangle $, and
% \begin{align}
% \label{eq:defrho}
%     \rho_t({r},y,F^{(1)},F^{(2)}) := \int_{0}^{r} F^{(2)}({z}-y)d{z} - r \left[ F^{(1)}({r}-y)\right]\,.
% \end{align}
% Note that $\expect_{\epsilon_t}\left[\max\{v_t^-, r \}\I\{v_t^+ > r\}\right] = \rho_t(r, y_t, F^-, F^+)$ for any $r\in\R$ that does not depend on $\left\{\epsilon_{i,t}\right\}_{i\in [N]}$ . Hence $\expect_{\epsilon_t}\left[\max\{v_t^-,r_t^\star \}\I\{v_t^+ > r_t^\star\}\right] = \rho_t(r_t^\star, y_t, F^-, F^+)$ and $\expect_{\epsilon_t}\left[\max\{v_t^-, \widehat{r}_t \}\I\{v_t^+ > \widehat{r}_t\}\right] = \rho_t(\widehat{r}_t, y_t, F^-, F^+)$ according to Proposition \ref{prop:benchmark}.  Also, defining $\widetilde{\mathcal{R}}_t^1 := \expect_{\epsilon_t}\left[\max\{v_t^-,r_t^\star \}\I\{v_t^+ > r_t^\star\} - \max\{v_t^-, \widehat{r}_t \}\I\{v_t^+ >  \widehat{r}_t\}\right]$,
%  Equation (\ref{eq:strat:boundR_t^11.5}) yields
%  \begin{align}
% \label{eq:strat:singleperiodregret1}
%      \mathcal{R}_t^{(1)}  ~ \leq ~ & \expect\left[\widetilde{\mathcal{R}}_t^1 \right] + \frac{v_{\max}}{|E_\ell|}
%  \end{align}

Then, we have
\begin{align}
   \mathcal{R}_t ~ = ~ &\rho_t(r_t^\star, y_t, F^-, F^+) - \rho_t(r_t, y_t, F^-, F^+) \nonumber \\
  ~ = ~ & \rho_t(r_t^\star, y_t, F^-, F^+) - \rho_t(r_t^\star, \widehat{y}_t,F^-, F^+) \nonumber \\
 & ~~ + \rho_t(r_t^\star, \widehat{y}_t, F^-, F^+) - \rho_t(r_t^\star, \widehat{y}_t, \widehat{F}_t^-, \widehat{F}_t^+) \nonumber \\
 & ~~ + \rho_t(r_t^\star, \widehat{y}_t, \widehat{F}_t^-, \widehat{F}_t^+) - \rho_t(r_t, \widehat{y}_t, \widehat{F}_t^-, \widehat{F}_t^+)\nonumber \\
  & ~~ +
  \rho_t(r_t, \widehat y_t, \widehat{F}_t^-, \widehat{F}_t^+) - \rho_t(r_t, \widehat{y}_t, F^-, F^+) \nonumber \\
  & ~~ + \rho_t(r_t, \widehat{y}_t , F^-, F^+) - \rho_t(r_t,y_t,F^-, F^+) \,. \label{eq:full:reg2}
\end{align}
We note that the second equation follows from adding and subtracting terms. Observe the first and the last terms of the second equation capture the impact of estimation error in the mean vector $
\beta$. Further, the second and forth terms  capture the impact of the estimation errors in distributions $F^-$ and $F^+$ while the third term captures the errors in reserve price with respect to all estimations. We now invoke  Lemma \ref{bound:controlUncert}, where we show that when events $\xi_t$, $\xi_t^-$, and $\xi_t^+$ happen, for $r \in \{r_t^\star, r_t\}$  we have 
\begin{enumerate}
    \item [(i)] $\left|\rho_t(r, y_t, F^-, F^+) - \rho_t(r, \widehat{y}_t, F^-, F^+)\right| ~ \leq ~ 3r c_f N^2 \delta_t$ a.s. 
    \item [(ii)]  $\left|\rho_t(r, y_t, F^-, F^+) - \rho_t(r, \widehat{y}_t, \widehat{F}_t^-, \widehat{F}_t^+) \right|~ \leq ~ r(3c_f N^2 \delta_t + 2\gamma_t)$ a.s.
\end{enumerate}
{This result relies on the Lipschitz properties of $F^-$ and $F^+$ shown in Lemma \ref{lemma:FF-F+Lipschitz}, and allows us to bound the regret using estimation errors without imposing the MHR assumption.}  Note that the first inequality bounds the impact of errors $\beta$ and the second bounds the impact of errors in the distributions.  Applying these bounds in (\ref{eq:full:reg2}), we get
\begin{align}
    & \mathcal{R}_t \cdot \I\{\xi_t \cap \xi_t^- \cap \xi_t^+\} \nonumber \\
    ~ \leq ~ &   3(r_t^\star + r_t)c_f N^2 \delta_t + \left(\rho_t(r_t^\star, \widehat{y}_t, \widehat{F}_t^-, \widehat{F}_t^+) - \rho_t(r_t, \widehat{y}_t, \widehat{F}_t^-, \widehat{F}_t^+) \right) +  (r_t^\star + r_t)\cdot (3c_f N^2 \delta_t + 2\gamma_t) \nonumber \\
      ~=~ &   2(r_t^\star + r_t)\cdot (3c_f N^2 \delta_t + \gamma_t) + \left(\rho_t(r_t^\star, \widehat{y}_t, \widehat{F}_t^-, \widehat{F}_t^+) - \rho_t(r_t, \widehat{y}_t, \widehat{F}_t^-, \widehat{F}_t^+) \right)\,. \label{eq:full:reg3}
\end{align}

We recall that the seller's pricing decision $r_t$ in period $t$ is defined in Equation (\ref{eq:reserve_price_1}), and observe that $r_t = \arg \max_{r\in [0, v_{\max}]}  \rho_t(r,\widehat{y}_t, \widehat{F}_t^-, \widehat{F}_t^+)$. Since $r_t^\star \in (0, v_{\max})$, we obtain the fact that $\rho_t(r_t^\star, \widehat{y}_t, \widehat{F}_t^-, \widehat{F}_t^+) - \rho_t(r_t, \widehat{y}_t, \widehat{F}_t^-, \widehat{F}_t^+)  \leq 0$. Plugging this into Equation (\ref{eq:full:reg3}), we get
\begin{align}
\label{eq:full:R_tfinal}
    \mathcal{R}_t \cdot \I\{\xi_t \cap \xi_t^- \cap \xi_t^+\} ~ \leq ~  2(r_t^\star + r_t)\cdot (3c_f N^2 \delta_t + \gamma_t)  ~ \leq ~ 4v_{\max} (3c_f N^2 \delta_t + \gamma_t) \,.
\end{align}

So far, we have bounded the single period regret for some period $t \in [T]$ assuming that events $\xi_t$, $\xi_t^-$, $\xi_t^+$ all hold. But, before we sum this regret up across all periods to get the cumulative regret, we first turn to upper bound the probability that not all of the events $\{\xi_t\}_{t \geq \TT}, \{\xi_t^-\}_{t\geq \TT}, \{\xi_t^+\}_{t \geq \TT}$ occur, where $\TT =\mathcal{O}(\sqrt{dT})$ is defined in Equation (\ref{eq:defTT}). We denote the complement of a set $\mathcal{A}$ to be $\mathcal{A}^c$. Hence, the probability that not all of the events $\{\xi_t\}_{t \geq \TT}, \{\xi_t^-\}_{t \geq \TT}, \{\xi_t^+\}_{t \geq \TT}$ occur is
%  Now, let $\TT =\left \lceil \max\left\{ \sqrt{dT}, \frac{2x_{max}^2\log(T)}{\lambda_0^2}, \exp\left(C\right), \tt \right\} \right \rceil + 1$, where $C = \frac{\epsilon_{max}^2 x_{max}^4}{N\lambda_0^4}$. \negin{We already defined $\TT$. Please use is here instead redefining it here.}  can be upper bounded as \negin{Please define the ``complement" operator. Note that the current notation is confusing because of all the constants }
\begin{align*}
     \prob\left( \bigcup_{t =\TT}^T  \left(\left\{\xi_t \right\}^c  \cup \left\{\xi_t^- \right\}^c \cup\left\{\xi_t^+ \right\}^c \right)\right)
    ~ \leq ~ \sum_{t =\TT}^T  \left[ \prob\left( \left\{\xi_t \right\}^c \right)+\prob\left( \left\{\xi_t^- \right\}^c \right)+\prob\left( \left\{\xi_t^+ \right\}^c \right)  \right]\,.
    % ~ = ~  & \sum_{t =\TT}^T \Big[ \prob\left( \left\{\xi_t \right\}^c \right) + \prob\left(\left\{\xi_t \right\} \cap \left\{\xi_t^- \right\}^c \right) + \prob\left(\left\{\xi_t \right\}^c \cap \left\{\xi_t^- \right\}^c \right)\\
    % & ~~ +\prob\left( \left\{\xi_t \right\} \cap \left\{\xi_t^+ \right\}^c   \right)+\prob\left( \left\{\xi_t \right\}^c \cap \left\{\xi_t^+ \right\}^c  \right)\Big] \\
    % ~ \leq ~ & \sum_{t =\TT}^T  \left[ \prob\left( \left\{\xi_t \right\}^c \right) + \prob\left(\left\{\xi_t \right\} \cap \left\{\xi_t^- \right\}^c \right) + \prob\left(\left\{\xi_t \right\}^c \right)+\prob\left( \left\{\xi_t \right\} \cap \left\{\xi_t^+ \right\}^c   \right)+\prob\left( \left\{\xi_t \right\}^c  \right)\right] \\
    % ~ = ~ & \sum_{t =\TT}^T  \left[ 3\prob\left( \left\{\xi_t \right\}^c \right)+\prob\left(\left\{\xi_t \right\} \cap \left\{\xi_t^- \right\}^c \right)+\prob\left( \left\{\xi_t \right\} \cap \left\{\xi_t^+ \right\}^c \right)  \right] .
\end{align*}
% The first inequality is due to the union bound, and the second inequality simply follows from the fact that $\left\{\xi_t \right\}^c \cap \left\{\xi_t^- \right\}^c \subseteq \left\{\xi_t \right\}^c$ and  $\left\{\xi_t \right\}^c \cap \left\{\xi_t^+ \right\}^c \subseteq \left\{\xi_t \right\}^c$. 
According to Lemma \ref{lemma:full:bias},  the probability $\prob\left( \left\{\xi_t \right\}^c \right)$ is bounded by
\begin{align}
    \label{eq:fullinfoprobbeta}
    \prob\left( \left\{\xi_t \right\}^c \right) ~ \leq ~ & \frac{2d}{(t-1)^2} + d\exp\left( - \frac{(t-1)\lambda_0^2}{8x_{\max}^2}\right)
    ~ \leq ~  \frac{2d}{(t-1)^2}+ \frac{d}{T^2},
\end{align}
where the second inequality is due to  our construction of $\TT$, such that for $t\geq \TT$ we have $t - 1 \geq 16 x_{\max}^2 \log(T)/\lambda_0^2$. On the other hand, by taking $\gamma = \gamma_t = \sqrt{2\log(t)}/\sqrt{t}$ in Lemma \ref{lemma:full:estimateF}, the probability $\prob\left(\left\{\xi_t^- \right\}^c \right)$ is bounded as:
% \begin{align}
%     \label{eq:fullinfoprobF}
%     & \prob\left(\left\{\xi_t \right\} \cap \left\{\xi_t^- \right\}^c \right) ~ \leq ~ \exp\left( -t\cdot \left( \frac{\sqrt{2\log(t)}}{\sqrt{t}} \right)^2\right) = \frac{4}{t^2}\\
%     & \prob\left(\left\{\xi_t \right\} \cap \left\{\xi_t^+ \right\}^c \right)~ \leq ~\exp\left( -t\cdot \left( \frac{\sqrt{2\log(t)}}{\sqrt{t}} \right)^2\right) = \frac{4}{t^2},
% \end{align}
\begin{align}
    % \label{eq:fullinfoprobF}
     \prob\left(\left\{\xi_t^- \right\}^c \right) ~ \leq ~ & 4\exp\left( -t\gamma^2\right) + \frac{4d}{(t-1)^2} +  2d\exp\left( - \frac{(t-1)\lambda_0^2}{8x_{\max}^2}\right)\nonumber\\
    ~ \leq ~ & 4\exp\left( -t\cdot \left( \frac{\sqrt{2\log(t)}}{\sqrt{t}} \right)^2\right)  + \frac{4d}{(t-1)^2}+ \frac{2d}{T^2}\nonumber\\
    ~ \leq ~ & \frac{4}{t^2} + \frac{4d}{(t-1)^2}+ \frac{2d}{T^2} \nonumber\,.
\end{align}
Similarly, we have $\prob\left(\left\{\xi_t^+ \right\}^c \right)~ \leq ~\frac{4}{t^2} + \frac{4d}{(t-1)^2}+ \frac{2d}{T^2}$. Therefore, 
\begin{align}
\nonumber
    \prob\left( \bigcup_{t =\TT}^\top  \left(\left\{\xi_t \right\}^c  \cup \left\{\xi_t^- \right\}^c \cup\left\{\xi_t^+ \right\}^c \right)\right)  ~ \leq ~ &\sum_{t = \TT}^\top  \left( \frac{5d}{T^2}+ \frac{10d}{(t-1)^2} + \frac{8}{t^2}\right)\\
    ~ \leq ~ & \int_{\sqrt{dT}}^\infty \frac{15d+8}{\tau^2}d\tau
     ~ \leq ~  \frac{23d}{\sqrt{dT}} =  \frac{23\sqrt{d}}{\sqrt{T}}. \label{eq:full:probCbound}
\end{align}
The second inequality is due to $\TT \geq \sqrt{dT}$ according to its definition, and the subsequent inequalities use the fact that $d\geq 1$. 

 Finally, we break down the cumulative expected regret into three parts: the trivial bound $v_{\max}$ for the regret from period $t =1 $ to $\TT-1$, the cumulative expected regret from period $t =\TT  $ to $T$ given the occurrence of events $\{\xi_t\}_{t \geq \TT}, \{\xi_t^-\}_{t \geq \TT}, \{\xi_t^+\}_{t \geq \TT}$, and the trivial bound from period $t =\TT  $ to $T$ if not all these events occur. Hence, the final cumulative regret is 
 \begin{align*}
     & \reg(T) \\
     ~ \leq ~ & v_{\max} \left(\TT -1\right) + \sum_{ t= \TT}^T \expect\left[\mathcal{R}_t \right] \\
      ~ = ~ & v_{\max} \left(\TT -1\right) + \sum_{ t= \TT}^T \expect\left[\mathcal{R}_t \cdot \I\{\xi_t \cap \xi_t^- \cap \xi_t^+\} \right] + \sum_{ t= \TT}^T \expect\left[\mathcal{R}_t \cdot \left(\I\left\{ \left(\xi_t\right)^c  \cup \left(\xi_t^- \right)^c \cup\left(\xi_t^+ \right)^c \right\}\right) \right] \\
     ~ \leq ~ & v_{\max} \left(\TT -1\right) + \sum_{ t= \TT}^T \expect\left[\mathcal{R}_t \cdot \left(\I\{\xi_t \cap \xi_t^- \cap \xi_t^+\} \right)\right] + T v_{\max} \prob\left( \bigcup_{t = \TT}^T  \left(\left(\xi_t \right)^c  \cup \left(\xi_t^- \right)^c \cup\left(\xi_t^+ \right)^c \right)\right) \\
      ~ \leq ~ & v_{\max} \TT + \sum_{ t= \TT}^T  4v_{\max} \left(3c_f N^2 \delta_t + \gamma_t\right)
     + T v_{\max} \cdot\prob\left( \bigcup_{t = \TT}^T  \left(\left(\xi_t \right)^c  \cup \left(\xi_t^- \right)^c \cup\left(\xi_t^+ \right)^c \right)\right)\\
      ~ \leq ~ & v_{\max}\TT + 4v_{\max} \sum_{ t= \TT}^T \left(3c_f N^2 \delta_t + \gamma_t\right)  +  T v_{\max} \cdot \frac{23\sqrt{d}}{\sqrt{T}}
 \end{align*}
 The first inequality applies Equation (\ref{eq:full:R_t0}) and uses the trivial bound $v_{\max}$ for each of the first $\TT$ periods; the second inequality is because $\mathcal{R}_t \leq v_{\max}$; the third inequality follows from Equations (\ref{eq:full:R_tfinal}), and the final inequality follows from (\ref{eq:full:probCbound}). Then, by plugging in the definition of $\delta_t$ and $\gamma_t$, 
%  \prob\left( \bigcup_{t = \TT}^T  \left(\left\{\xi_t \right\}^c  \cup \left\{\xi_t^- \right\}^c \cup\left\{\xi_t^+ \right\}^c \right)\right)  \leq 1
 \begin{align}
     & \reg(T) \nonumber\\
     ~ \leq ~ & v_{\max}\TT + 4v_{\max} \int_{0}^T \left(3c_f N^2 \cdot \frac{4\sqrt{d\log(\tau)}\epsilon_{\max} x_{\max}^2}{\lambda_0^2\sqrt{N\tau}} + \frac{\sqrt{2\log(\tau)}}{\sqrt{\tau}}\right)d\tau  +  23v_{\max} \sqrt{dT} \nonumber\\
    ~ \leq ~ &  v_{\max}\TT + 4v_{\max} \left( \frac{24c_f\epsilon_{\max} x_{\max}^2  \sqrt{dN^3T\log(T)}}{\lambda_0^2} + 2\sqrt{2T\log(T)} \right) +  23 v_{\max}\sqrt{dT} \nonumber\\
   ~ = ~ & \mathcal{O}\left(c_f\sqrt{dN^3 T\log(T)}\right)  \nonumber \,,
 \end{align}
 where the first inequality follows from the fact that a summation of monotonically decreasing functions can be upper bounded by its integral.

\subsection{Other Lemmas for proving Theorem \ref{bound:fullInfoRegret}} \label{appsec:truthfullotherlem}

\begin{lemma}[Bounding Estimation Errors in $F^-$ and $F^+$] \label{lemma:full:estimateF} {Define $\sigma_t$ to be the sigma algebra generated by all $\{x_\tau\}_{\tau \in[t]} $ and $\{\epsilon_{i,\tau}\}_{i\in [N],\tau \in[t]} $.}  Then, for any $\sigma_t$-measurable random variable ${z}$ and any $\gamma> 0$, we have 
\begin{align*}
    \prob\left( \left|F^-(z)-  \widehat{F}_t^-(z) \right| \leq \gamma + 2c_f N^2\delta_t \right) ~ \geq ~  1 - 4\exp\left( -t\gamma^2\right) - \frac{4d}{(t-1)^2}-  2d\exp\left( -\frac{(t-1)\lambda_0^2}{8x_{\max}^2}\right)\, \text{ and}
\end{align*}
\begin{align*}
    \prob\left( \left|F^+(z)-  \widehat{F}_t^+(z) \right| \leq \gamma + c_f N\delta_t \right) ~ \geq ~  1 - 4\exp\left( -t\gamma^2\right) - \frac{4d}{(t-1)^2}-  2d\exp\left( -\frac{(t-1)\lambda_0^2}{8x_{\max}^2}\right)\,,
\end{align*}
{where $\delta_{t} = \frac{4\sqrt{d\log(t-1)}\epsilon_{\max} x_{\max}^2}{\lambda_0^2\sqrt{N(t-1)}}$, $c_f = \sup_{{z}\in [-\epsilon_{\max},\epsilon_{\max}]}f(z)$, and $\lambda_0^2 > 0$ is the smallest eigenvalue of $\Sigma = \expect_{x\sim\mathcal{D}}[xx^T]$.}
\end{lemma}

\begin{proof}
Our goal here is to show that $\big|F^-(z)-  \widehat{F}_t^-(z) \big|$ is small with high probability. According to our estimate of $F^-$ in NPAC-T policy,
    \begin{align*}
        \widehat{F}_t^-({z}) ~ = ~ & \frac{1}{t-1} \sum_{\tau \in [t-1]} \I\left\{ v_\tau^- -\langle  \widehat{\beta}_t, x_\tau \rangle \leq {z} \right\}\\
         ~ = ~ & \frac{1}{t-1} \sum_{\tau \in [t-1]} \I\left\{ \epsilon_\tau^- \leq {z} + \langle  \widehat{\beta}_{t} - \beta, x_\tau \rangle\right\}\,.
     \end{align*}
We highlight that $\expect\left[\widehat{F}_t^-({z}) \right] \ne \frac{1}{t-1} \sum_{\tau \in [t-1]} F^-\left({z} + \langle  \widehat{\beta}_{t} - \beta, x_\tau \rangle \right)$ because both $z$ and $\widehat{\beta}_{t}$ are $\sigma_t$-measurable. Hence,  one cannot naively apply concentration inequalities to bound $\Big|F^-(z)-  \widehat{F}_t^-(z) \Big|$. Therefore, our approach is to first construct upper and lower bounds for $\widehat{F}_t^-({z})$ that are not functions of $\widehat{\beta}_t$,  and then apply concentration inequalities on these upper and lower bounds respectively.
 
Recall the definition of the event $\xi_t = \left\{\norm{\widehat{\beta}_t - \beta}_1 \leq {\delta_t}/{x_{\max}} \right\}$. Under this event, we have
     \begin{align}
         \frac{1}{t-1} & \sum_{\tau \in [t-1]} \I\left\{ \epsilon_\tau^- \leq {z} - \delta_t \right\} ~ \leq ~ \widehat{F}_t^-({z}) ~ \leq ~ \frac{1}{t-1} \sum_{\tau \in [t-1]} \I\left\{ \epsilon_\tau^- \leq {z} + \delta_t \right\}\,. \label{eq:F}
     \end{align}
%where this holds because the occurrence of the event $\xi_t$.
Now,  for  any $\gamma > 0$,  we have 
\begin{align*}
    & \prob\left( \widehat{F}_t^-({z}) - F^-({z} + \delta_t) \leq \gamma \right) \\
    ~ \geq ~ &  \prob\left( \left\{\widehat{F}_t^-({z}) - F^-({z} + \delta_t) \leq \gamma\right\} ~ \bigcap ~ \xi_t \right) \\
    ~ \geq ~ &  \prob\left( \left\{\frac{\sum_{\tau \in [t-1]} \I\left\{ \epsilon_\tau^- \leq{z} + \delta_t \right\}}{t-1} - F^-({z} + \delta_t)  \leq \gamma \right\} ~ \bigcap ~ \xi_t \right)\\
   ~ \geq ~ & \prob\left( \left\{ \sup_{\Tilde{{z}} \in \R} \Big| \frac{1}{t-1} \sum_{\tau \in [t-1]} \I\left\{ \epsilon_\tau^- \leq \Tilde{{z}} \right\} - F^-(\Tilde{{z}}) \Big| \leq \gamma \right\} ~ \bigcap \xi_t \right)\\
    ~ \geq ~ & 1 - \prob\left(\sup_{\Tilde{{z}} \in \R} \Big| \frac{1}{t-1} \sum_{\tau \in [t-1]} \I\left\{ \epsilon_\tau^- \leq \Tilde{{z}} \right\} - F^-(\Tilde{{z}}) \Big| > \gamma \right) - \prob\left(\xi_t^c \right)\\
     ~ \geq ~ & 1 - 2\exp\left( -2(t-1)\gamma^2\right) - \frac{2d}{(t-1)^2}-  d\exp\left( -\frac{(t-1)\lambda_0^2}{8x_{\max}^2}\right)\\
      ~ \geq ~ & 1 - 2\exp\left( -t\gamma^2\right) - \frac{2d}{(t-1)^2}-  d\exp\left( -\frac{(t-1)\lambda_0^2}{8x_{\max}^2}\right) \,,
    % ~ \geq ~ & 1 - 2\exp\left( -t\gamma^2\right) - \frac{8d}{t^2}-  d\exp\left( -\frac{t\lambda_0^2}{16x_{\max}^2}\right) \,,
\end{align*}
where the second inequality follows from (\ref{eq:F}), the fourth inequality follows from the union bound, and the second last inequality follows from the Dvoretzky-Kiefer-Wolfowitz (DKW) inequality (Theorem \ref{DKW}) and Lemma \ref{lemma:full:bias}. We note that we can apply the DKW inequality because   $\{\epsilon_\tau^-\}_{\tau\in[t-1]}$ are $t-1$ i.i.d. realizations of the $(N-1)^{th}$ order statistic of $N$ i.i.d. noise variables. The last inequality holds  because $t \geq 2$ and as a result,  $t-1 \geq \frac{t}{2}$. Furthermore, invoking the Lipschitz properties of $F^-$ shown in Lemma \ref{lemma:FF-F+Lipschitz}, we have $|F^-({z} + \delta_t) - F^-({z})| \leq 2  c_f N^2 \delta_t$.  Therefore, 
\begin{align}
\label{eq:F-1}
    & \prob\left( \widehat{F}_t^-({z}) - F^-({z}) ~ \leq ~ \gamma + 2c_f N^2 \delta_t\right) \nonumber \\
    ~ \geq ~ &  \prob\left( \widehat{F}_t^-({z}) - F^-({z} + \delta_t) \leq \gamma \right) \nonumber\\
    ~ \geq ~ & 1 - 2\exp\left( -t\gamma^2\right) - \frac{2d}{(t-1)^2}-  d\exp\left( -\frac{(t-1)\lambda_0^2}{8x_{\max}^2}\right)\,.
\end{align}
Similarly, we have  $|F^-({z})-F^-({z} - \delta_t)| \leq 2c_f N^2 \delta_t$ by Lemma \ref{lemma:FF-F+Lipschitz}. Hence, following the same arguments as in the case of $\prob\left( \widehat{F}_t^-({z}) - F^-({z}) ~ \leq ~ \gamma + 2c_f N^2 \delta_t\right)$, we have 
\begin{align}
\label{eq:F-2}
    \prob\left(  F^-({z})-  \widehat{F}_t^-({z})  \leq \gamma + 2c_f N^2\delta_t \right)
     ~ \geq ~ & \prob\left(  F^-({z} - \delta_t)-  \widehat{F}_t^-({z}) \leq \gamma \right) \nonumber \\
     ~ \geq ~ & 1 - 2\exp\left( -t\gamma^2\right) - \frac{2d}{(t-1)^2}-  d\exp\left( -\frac{(t-1)\lambda_0^2}{8x_{\max}^2}\right)\,.
\end{align}
{Finally, applying a union bound on Equations (\ref{eq:F-1}) and (\ref{eq:F-2}) will yield the result in the statement of the lemma. We can show a similar result for  $F^+({z})-  \widehat{F}_t^+({z}) $ by following the same reasoning.}
\end{proof}

\begin{lemma}[Lipschitz Property for $F$, $F^-$ and $F^+$]\label{lemma:FF-F+Lipschitz}
The following hold for any ${z}_1, {z}_2 \in \R$:
\begin{enumerate}
    \item [(i)]  $|F({z}_1) -  F({z}_2)| \leq c_f |{z}_1-{z}_2 |$.
    \item [(ii)] $|F^-({z}_1) -  F^-({z}_2)| \leq 2c_f N^2|{z}_1-{z}_2 |$.
    \item [(iii)]$|F^+({z}_1) -  F^+({z}_2)| \leq c_f N|{z}_1-{z}_2 |$.
\end{enumerate}
Here,  $0<c_f = \sup_{{z}\in [-\epsilon_{\max},\epsilon_{\max}]}f(z)$.
\end{lemma}

\textit{Proof of Lemma \ref{lemma:FF-F+Lipschitz}.}
Without loss of generality, we assume ${z}_1 < {z}_2$. Note that $F({z}) = 0$ for $\forall {z}\in (-\infty, -\epsilon_{\max}]$, and $F({z}) = 1$ for $\forall {z}\in [\epsilon_{\max}, \infty)$.

\textbf{Part (i)}
We consider the following cases:
\begin{enumerate}\label{eq:LipschitzF}
    \item [Case 1:]  $\left({z}_1 < {z}_2 \leq - \epsilon_{\max} ~ \text{ or } ~ \epsilon_{\max} \leq {z}_1 < {z}_2 \right)$: $|F({z}_2) - F({z}_1)| = 0 \leq c_f|{z}_2 - {z}_1|$.
     \item [Case 2:]  $\left(-\epsilon_{\max} < {z}_1 < {z}_2 < \epsilon_{\max}\right)$: By the mean value theorem,  $|F({z}_2) - F({z}_1)| = f({\tilde{z}}) |{z}_2 - {z}_1| < c_f |{z}_2 - {z}_1|$, where $\tilde{z} \in ({z}_1, {z}_2)$.
    \item [Case 3:]  $\left( {z}_1 \leq -\epsilon_{\max} < {z}_2 < \epsilon_{\max}\right)$: We have $|{z}_2 - (-\epsilon_{\max})| = {z}_2  - (-\epsilon_{\max}) \leq {z}_2 - {z}_1$ and  $F({z}_1) = F(-\epsilon_{\max}) = 0$. Hence $|F({z}_2) - F({z}_1)| = |F({z}_2) - F(-\epsilon_{\max})| = f({\tilde{z}}) |{z}_2 - (-\epsilon_{\max})| \leq c_f|{z}_2 - {z}_1|$, where $\tilde{z} \in (-\epsilon_{\max}, {z}_2)$ by the mean value theorem. 
    \item [Case  4]  $\left(-\epsilon_{\max} < {z}_1 <  \epsilon_{\max} \leq {z}_2 \right)$: We have $|\epsilon_{\max}- {z}_1| = \epsilon_{\max}- {z}_1 \leq  {z}_2 - {z}_1$ and $F({z}_2) = F(\epsilon_{\max}) =1 $ . Hence $|F({z}_2) - F({z}_1)| = |F(\epsilon_{\max}) - F({z}_1) | = f({\tilde{z}}) |\epsilon_{\max}- {z}_1|  \leq c_f |{z}_2 - {z}_1|$, where $\tilde{z} \in ({z}_1, \epsilon_{\max})$ by the mean value theorem. 
\end{enumerate}

\textbf{Part (ii) \& (iii)}
We recall that $F^-({z}) = NF^{N-1}({z}) - (N-1)F^N({z})$ and $F^+({z}) = F^N({z})$, so
 \begin{align} 
    &  |F^-({z}_2) - F^-({z}_1)| \nonumber \\
    ~ = ~ &  \left|NF^{N-1}({z}_2)- (N-1)F^{N}({z}_2)- \left(NF^{N-1}({z}_1)- (N-1)F^{N}({z}_1)\right)\right| \nonumber \\
     ~ \leq ~ &  N\left|F^{N-1}({z}_2) - F^{N-1}({z}_1) \right| + (N-1)\left| F^{N}({z}_2) -F^{N}({z}_1)\right| \nonumber \\
    ~ = ~ &  N\left|\left(F({z}_2) - F({z}_1)\right)\left(\sum_{n = 1}^{N-1} \left(F({z}_2)\right)^{n-1}\left(F({z}_1)\right)^{N -1 - n} \right) \right|\nonumber \\
    & ~~~ + (N-1)\left|\left(F({z}_2) - F({z}_1)\right)\left(\sum_{n = 1}^{N} \left(F({z}_2)\right)^{n-1}\left(F({z}_1)\right)^{N - n} \right) \right| \nonumber \\ 
    ~ \leq ~ & N(N-1) \left|F({z}_2) - F({z}_1) \right| + (N-1)N\left |F({z}_2) - F({z}_1)\right| \nonumber\\
    ~ < ~ & 2N^2 c_f |{z}_2 - {z}_1| \nonumber \,.
\end{align}
 The second equality uses $a^m - b^m = (a-b)\left(\sum_{n = 1}^m a^{n-1} b^{m - n} \right)$ for any $a,b \in \R$ and integer $m \geq 2$. The second inequality follows from $F({z}) \in [0,1]$ for $\forall {z} 
 \in \R$. The final inequality follows from the Lipschitz property of $F$ shown in part (i). Following the same arguments, we can also show that $|F^+({z}_2) - F^+({z}_1)| \leq  c_f N|{z}_2 - {z}_1|$. 
 \endproof 

% \begin{lemma}[Bounding Estimation Errors in $F^-$ and $F^+$] \label{lemma:full:estimateF} {Define $\sigma_t$ to be the sigma algebra generated by all $\{x_\tau\}_{\tau \in[t]} $ and $\{\epsilon_{i,\tau}\}_{i\in [N],\tau \in[t]} $.}  Then, for any $\sigma_t$-measurable random variable ${z}$ and any $\gamma> 0$, we have 
% \begin{align*}
%     \prob\left( \left|F^-(z)-  \widehat{F}_t^-(z) \right| \leq \gamma + 2c_f N^2\delta_t \right) ~ \geq ~  1 - 4\exp\left( -t\gamma^2\right) - \frac{4d}{(t-1)^2}-  2d\exp\left( -\frac{(t-1)\lambda_0^2}{8x_{\max}^2}\right)\, \text{ and}
% \end{align*}
% \begin{align*}
%     \prob\left( \left|F^+(z)-  \widehat{F}_t^+(z) \right| \leq \gamma + c_f N\delta_t \right) ~ \geq ~  1 - 4\exp\left( -t\gamma^2\right) - \frac{4d}{(t-1)^2}-  2d\exp\left( -\frac{(t-1)\lambda_0^2}{8x_{\max}^2}\right)\,,
% \end{align*}
% {where $\delta_{t} = \frac{4\sqrt{d\log(t-1)}\epsilon_{\max} x_{\max}^2}{\lambda_0^2\sqrt{N(t-1)}}$ and $c_f = \sup_{{z}\in [-\epsilon_{\max},\epsilon_{\max}]}f(z)$.}
% \end{lemma}

\begin{lemma}[Bounding Estimation Errors in $\beta$]
\label{lemma:full:bias} For any $\gamma > 0$,
\begin{align*}
  \prob\left( \norm{\widehat{\beta}_{t+1} - \beta}_1 \leq \gamma \right) ~ \geq ~ & 1 -  2d\exp\left( -\frac{N\gamma^2\lambda_0^4 t }{8 \epsilon_{\max}^2x_{max}^2 d}\right)  -  d\exp\left( -\frac{t\lambda_0^2}{8x_{max}^2}\right)\,,
\end{align*} where $\lambda_0^2$ is the minimum eigenvalue of covariance matrix $\Sigma$ and the estimate $\widehat{\beta}_{t+1}$ is defined in Equation (\ref{eq:fullinfobetaestimate}). Furthermore, setting $\gamma =  \frac{4\sqrt{d\log(t)}\epsilon_{\max} x_{\max}}{\lambda_0^2\sqrt{Nt}}$ and denoting $\delta_{t+1} = \gamma  x_{\max}$, we have 
\begin{align*}
    \prob\left( \norm{\widehat{\beta}_{t+1} - \beta}_1 \leq \frac{\delta_{t+1}}{x_{\max}} \right) \geq 1 - \frac{2d}{t^2}-  d\exp\left( -\frac{t\lambda_0^2}{8x_{\max}^2}\right)\,.
\end{align*}
\end{lemma}

\textit{Proof of Lemma \ref{lemma:full:bias}.}

The proof of Lemma \ref{lemma:full:bias} is inspired by Lemma EC.7.2  in \cite{bastani2015online}.
% We will show that for any  $\gamma > 0$, with probability at least
% $1 -  2d\exp\left( -\frac{N\gamma^2\lambda_0^4 t }{2\epsilon_{max}^2x_{max}^2 d}\right)  -  d\exp\left( -\frac{t\lambda_0^2}{2x_{max}^2}\right)$, we have $\norm{\widehat{\beta}_{t+1} - \beta}_1 \leq \gamma$. Hence,  by taking $\gamma =  \frac{\delta_{t+1}}{x_{max}} = \frac{2\sqrt{d}\log(t)}{x_{max}\sqrt{t} }$, we get the desired result. 
First, recall that the smallest eigenvalue $\lambda_0^2$ of the covariance matrix $\Sigma$ of $x\sim \mathcal{D}$ is greater than $0$. Since the second moment matrix $\expect[x_t x_t^\top] = \Sigma + \expect[x] \expect[x]^\top$, we know that the smallest eigenvalue of $\expect[x_t x_t^\top]$ is at least $\lambda_0^2 > 0$. We  denote the design matrix of all the features up to time $t$ as $X$ where $X\in \R^{t \times d}$, and $\Bar{\epsilon}_\tau = \frac{\sum_{i\in[N]}\epsilon_{i,\tau}}{N}$ for $\forall \tau \in [t]$. 
 
 We first consider the case where the smallest eigenvalue of the second moment matrix $\lambda_{\min}\left( X^\top  X/t \right) \geq \lambda_0^2/2$, which implies that $(X^\top X)^{-1}$ exists and $(X^\top X)^{-1} = (X^\top X)^\dag$ . Later, we show that with high probability, $\lambda_{\min}\left( X^\top  X/t\right) \geq \lambda_0^2/2$.
By the definition of $\widehat{\beta}_{t+1}$ and $\Bar{v}_t$ in Equations (\ref{eq:fullinfobetaestimate}), 
 \begin{align}
     \widehat{\beta}_{t+1} = \left(X^\top X \right)^{-1} X^\top  \left(\begin{matrix}\Bar{v}_1\\ \vdots\\ \Bar{v}_t \nonumber \\ \end{matrix}\right) &= \left(X^\top X \right)^{-1} X^\top  \left(\begin{matrix} \frac{\sum_{i\in[N]} v_{i,1}}{N}\\ \vdots\\ \frac{\sum_{i\in[N]} v_{i,t}}{N}\\ \end{matrix}\right)  \nonumber\\
     & =\beta +\left(X^\top X \right)^{-1} X^\top   \left(\begin{matrix} \frac{\sum_{i\in[N]} \epsilon_{i,1}}{N}\\ \vdots\\ \frac{\sum_{i\in[N]} \epsilon_{i,t}}{N}\\ \end{matrix}\right)  \nonumber\\
     & = \beta +\left(X^\top X \right)^{-1} X^\top \Bar{\mathcal{E}}\nonumber \,,
 \end{align}
 where $\Bar{\mathcal{E}}$  is the column vector consisting of all $\Bar{\epsilon}_\tau = \frac{\sum_{i\in[N]}\epsilon_{i,\tau}}{N}$ for $\forall \tau \in [t]$. Therefore, 
\begin{align}
\label{eq:full:biasbound2norm}
    \norm{\widehat{\beta}_{t+1} - \beta}_2  = \norm{\left(X^\top X \right)^{-1} X^\top  \Bar{\mathcal{E}}}_2 
    \leq  \frac{2}{t\lambda_0^2}\cdot \norm{X^\top  \Bar{\mathcal{E}}}_2\,,
\end{align}
since we assumed $\lambda_{\min}\left( X^\top  X/t\right) \geq \lambda_0^2/2$. Denote $X^j$ as the $j$th column of $X$, i.e., the 
$j$th row of $X^\top $, for $j = 1,2\dots d$. Since $ \norm{X^\top  \Bar{\mathcal{E}}}_2^2 = \sum_{j\in[d]}  \left| \Bar{\mathcal{E}}^\top  X^j  \right|^2 $, for any $\gamma > 0$ we have 
\begin{align}
\label{eq:full:biasbound2norm_2}
     \bigcap_{j \in [d]} \left\{ \left| \Bar{\mathcal{E}}^\top  X^j  \right|  ~ \leq ~ \frac{t\lambda_0^2\gamma }{2\sqrt{d}} \right\} \subseteq \left\{ \frac{2}{t\lambda_0^2}\cdot  \norm{X^\top  \Bar{\mathcal{E}}}_2 \leq \gamma \right\}\,.
\end{align}
We observe that $ \Bar{\mathcal{E}}^\top  X^j = \frac{\sum_{\tau\in E_\ell}\sum_{i\in [N]}\epsilon_{i,\tau}X_{\tau j}}{N}$, where all $\epsilon_{i,\tau}X_{\tau j}$ are $0$-mean and ${\epsilon_{\max}} x_{\max}$-subgaussion \footnote{{A random variable $Z$ is $\sigma$-subgaussian if for $\forall{\gamma}\in \R$, $\expect[\exp(\gamma Z)] \leq \exp(\gamma^2 \sigma^2/2)$.}} random variables. {Therefore by Hoeffding's inequality, for any $\tilde{\gamma} > 0$}
\begin{align}
\label{eq:full:biasbound2norm_3}
    & \prob\left( \left|N\Bar{\mathcal{E}}^\top  X^j \right| \leq \Tilde{\gamma} \right) \geq 1 - 2\exp\left( -\frac{ \Tilde{\gamma}^2}{2{\epsilon_{\max}^2}x_{max}^2 tN}\right)\,.
\end{align}

% \begin{align}
%   & \prob\left( \left|\mathcal{E}^\top  X^j \right| \leq \frac{t\lambda_0^2\gamma }{\sqrt{d}}  \right) \geq 1 - 2\exp\left( -\frac{N\gamma^2\lambda_0^4 t }{2{\epsilon_{\max}}^2x_{max}^2 d}\right)\,, \label{eq:full_hoeffding}
% \end{align}
Hence, 
\begin{align}
\label{eq:full:biasbound2norm_4}
     \prob\left( \frac{2}{t\lambda_0^2}\cdot  \norm{X^\top  \Bar{\mathcal{E}}}_2 \leq \gamma \right) 
    ~ \geq ~   &\prob\left(\bigcap_{j \in [d]} \left\{ \left| \Bar{\mathcal{E}}^\top  X^j  \right|  \leq \frac{t\lambda_0^2\gamma }{2\sqrt{d}} \right\}\right) \nonumber\\
    ~\geq ~ & 1 - \sum_{j\in [d]} \prob\left( \left| \Bar{\mathcal{E}}^\top  X^j  \right| > \frac{t\lambda_0^2\gamma }{2\sqrt{d}} \right) \nonumber \\
     ~\geq ~ & 1 -  2d\exp\left( -\frac{N\gamma^2\lambda_0^4 t }{8\epsilon_{\max}^2x_{\max}^2 d}\right) \,,
\end{align}
where the first inequality follows from Equation (\ref{eq:full:biasbound2norm_2}), the second inequality applies the union bound, and the last inequality follows from Equation (\ref{eq:full:biasbound2norm_3}) by
replacing  $\tilde{\gamma}$ with $N t\lambda_0^2\gamma /(2\sqrt{d})$.

Now it only remains to show $\lambda_{\min}\left(X^\top  X/t\right) \geq \lambda_0^2/2$ with high probability, which can be achieved by applying Lemma \ref{matrixchernoff}. In the context of this lemma, we consider the sequence of random matrices $\{ x_\tau x_\tau^\top /t\}_{\tau\in[t]}$, and note that $X^\top X/t = \sum_{\tau\in[t]} (x_\tau x_\tau^\top /t)$.  We first  upper bound the maximum eigenvalue of $x_\tau x_\tau^\top /t$, namely $\lambda_{\max}\left(x_\tau x_\tau^\top /t\right) $ for any $\tau \in [t]$ by 
\begin{align}
% \label{eq:boundmaxeigenvalue}
    \lambda_{\max}\left(\frac{x_\tau x_\tau^\top}{t} \right)  = \max_{\norm{z}_2 =1} z^\top \frac{x_\tau x_\tau^\top}{t} z \leq \frac{1}{t} \max_{\norm{z}_2 =1}(x^\top z)^2 \leq \frac{x_{\max}^2}{t} \nonumber \,.
\end{align}
 This allows us to apply Lemma \ref{matrixchernoff} (setting $\Bar{\gamma} = 1/2$ in the lemma) and get
\begin{align}
\label{eq:full:matrixchernoff}
   \prob\left(\lambda_{\min}\left(\frac{X^\top X}{t} \right) \geq  \frac{\lambda_0^2}{2} \right) ~ \geq ~ & \prob\left(\lambda_{\min}\left(\frac{X^\top X}{t} \right)  \geq ~ \frac{\lambda_{\min}\left(\expect[X^\top X/t]\right)^2}{2} \right) \nonumber\\
   ~ \geq ~ &  1- d\exp\left( -\frac{t\lambda_0^2}{8x_{max}^2}\right)\,,
\end{align} 
where  the first inequality follows from the fact that $\lambda_{\min}\left(\expect[X^\top X/t]\right) \geq \lambda_0^2$.

Therefore, 
\begin{align*}
     \prob\left( \norm{\widehat{\beta}_{t+1} - \beta}_1 \leq \gamma \right)
     ~\geq ~&\prob\left( \norm{\widehat{\beta}_{t+1} - \beta}_2 \leq \gamma \right)\\
      ~\geq ~ &
    \prob\left(\left\{ \frac{2}{t\lambda_0^2}\cdot  \norm{X^\top  \Bar{\mathcal{E}}}_2 \leq \gamma \right\}  \bigcap \left\{\lambda_{\min}\left(\frac{X^\top X}{t} \right) \geq   \frac{\lambda_0^2}{2}\right\}\right) \\
    % ~\geq ~ &  \prob\left(\bigcap_{j \in [d]} \left\{ \left| \mathcal{E}^\top  X^j  \right|  \leq \frac{t\lambda_0^2\gamma }{\sqrt{d}} \right\}  \bigcap \left\{\lambda_{\min}\left(\frac{X^\top X}{t} \right) \geq  \frac{\lambda_0^2}{2}\right\}\right) \\
    % ~\geq ~ & 1 - \sum_{j\in [d]} \prob\left( \left| \mathcal{E}^\top  X^j  \right| > \frac{t\lambda_0^2\gamma }{\sqrt{d}} \right)  - \prob\left( \lambda_{\min}\left(\frac{X^\top X}{t} \right) < \frac{\lambda_0^2}{2} \right) \\
     ~\geq ~ & 1 - \prob\left(\frac{2}{t\lambda_0^2}\cdot  \norm{X^\top  \Bar{\mathcal{E}}}_2 > \gamma \right)  - \prob\left( \lambda_{\min}\left(\frac{X^\top X}{t} \right) < \frac{\lambda_0^2}{2} \right) \\
     ~\geq ~ & 1 -  2d\exp\left( -\frac{N\gamma^2\lambda_0^4 t }{8 \epsilon_{\max}^2x_{max}^2 d}\right)  -  d\exp\left( -\frac{t\lambda_0^2}{8x_{max}^2}\right)\,.
     \end{align*}
{The first inequality follows from the fact that $\norm{{z}}_1 \leq \norm{{z}}_2$ for any vector ${z}$; the second inequality follow from Equation (\ref{eq:full:biasbound2norm}); the fourth inequality applies a simple union bound; and the final inequality follows from Equations (\ref{eq:full:biasbound2norm_4}) and (\ref{eq:full:matrixchernoff}).} 
 \endproof

 {The following Lemma utilizes the Lipschitz properties of $F^-$ and $F^+$ shown in Lemma \ref{lemma:full:estimateF} to bound the seller's regret in terms of the estimation errors of both $\beta$, $F^-$ and $F^+$.}
 \begin{lemma}[Bounding the Impact of Estimation Errors on Revenue]  \label{bound:controlUncert}
Assume that the events $\xi_t = \left\{\norm{\widehat{\beta}_t - \beta}_1 \leq {\delta_t}/{x_{max}} \right\}$, $\xi_t^- = \left\{\left|F^-({z})-  \widehat{F}_t^-({z}) \right| \leq \gamma_t + 2c_f N^2\delta_t ~~ \text{for } \forall {z} \in\R \right\}$ and $\xi_t^+ = \left\{\left|F^+({z})-  \widehat{F}_t^+({z}) \right| \leq \gamma_t + c_f N \delta_t ~~ \text{for } \forall {z} \in\R  \right\}$ occur with $\gamma_t = \sqrt{2\log(t)}/\sqrt{t} $, and $\delta_t =  \frac{4\sqrt{d\log(t-1)}\epsilon_{\max} x_{\max}^2}{\lambda_0^2\sqrt{N(t-1)}} $. Then,  for ${r} \in \{r_t^\star, r_t\}$ we have the following:
\begin{enumerate}
    \item [(i)] $\left|\rho_t(r, y_t, F^-, F^+) - \rho_t(r, \widehat{y}_t, F^-, F^+)\right| \leq 3r c_f N^2 \delta_t$ a.s. 
    \item [(ii)] $\left|\rho_t(r, y_t, F^-, F^+) - \rho_t(r, \widehat{y}_t, \widehat{F}_t^-, \widehat{F}_t^+) \right|\leq r(3c_f N^2 \delta_t + 2\gamma_t)$ a.s.
\end{enumerate}
where $y_t = \langle \beta, x_t \rangle$, $\widehat{y}_t = \langle  \widehat{\beta}_t, x_t \rangle$, $\widehat{\beta}_t,\widehat{F}_t^-, \widehat{F}_t^+$ are defined in Equations (\ref{eq:fullinfobetaestimate}) and (\ref{eq:fullinfoalgoFestimate}). The function $\rho_t$ is defined in Equation (\ref{eq:defrho}).
\textit{Proof of Lemma \ref{bound:controlUncert}.}
\textbf{Part (i)} We consider the following:
 \begin{align*}
     &\left|\rho_t(r, y_t, F^-, F^+) - \rho_t(r, \widehat{y}_t, F^-, F^+)\right| \\
     ~ = ~& \left| \int_{0}^r \left[F^-({z}-y_t )-F^-({z}- \widehat{y}_t ) \right]d{z} - r \left[ F^+(r-y_t)-F^+(r- \widehat{y}_t)\right] \right| \\
     ~ \leq ~ &  \int_{0}^r \left|F^-({z}-y_t )-F^-({z}- \widehat{y}_t ) \right| d{z} + r \left| F^+(r-y_t)-F^+(r- \widehat{y}_t)\right| \\
     ~ \leq ~ &  \int_{0}^r 2c_f N^2 |y_t - 
     \widehat{y}_t| d{z} + r c_f N |y_t - 
     \widehat{y}_t|\\
      ~ \leq ~  &  \int_{0}^r 2c_f N^2 \left(\norm{\widehat{\beta}_{t} - \beta}_1 x_{\max}\right)d{z} + r c_f N \norm{\widehat{\beta}_{t} - \beta}_1 x_{\max } \\
     ~ < ~ & 3r c_f N^2  \delta_t\,.
 \end{align*} The first equality follows from definition of $\rho_t$ in Equation \ref{eq:defrho};
  the second inequality follows from Lemma \ref{lemma:FF-F+Lipschitz}, the  third inequality follows from Cauchy's inequality: $|y_t - \widehat{y}_t| = |\langle \widehat{\beta}_{\ell+1} - \beta, x_t \rangle| \leq \norm{\widehat{\beta}_{\ell+1} - \beta}_1 x_{\max}$, and the last inequality follows from the occurrence of the occurrence of $\xi_t$ and $N\geq 1$.

\textbf{Part (ii)} Similar to part (i), we have 
 \begin{align*}
     &\left|\rho_t(r,\widehat{y}_t, F^-, F^+) - \rho_t(r, \widehat{y}_t, \widehat{F}_t^-, \widehat{F}_t^+)\right| \\
     ~ = ~ &\left| \int_{0}^r \left[F^-({z}-\widehat{y}_t )- \widehat{F}_t^-({z}- \widehat{y}_t ) \right]d{z} - r \left[ F^+(r-\widehat{y}_t)- \widehat{F}_t^+(r- \widehat{y}_t)\right] \right| \\
     ~ \leq ~ &  \int_{0}^r \left|F^-({z}-\widehat{y}_t )- \widehat{F}_t^-({z}- \widehat{y}_t ) \right| d{z} + r \left| F^+(r-\widehat{y}_t)- \widehat{F}_t^+(r- \widehat{y}_t)\right| \\
     ~ < ~ & r (3c_f N^2 \delta_t + 2\gamma_t)\,.
 \end{align*}
 where the last inequality follows from the occurrence of events $\xi_t^-$ and $\xi_t^+$, and $N\geq 1$. 
\endproof
\end{lemma}
